# Supplementary material for: Why Fe$_3$GaTe$_2$ has higher Curie temperature than Fe$_3$GeTe$_2$?
Source: arXiv:2504.17998 source file (2025-04-25)
Supplement: Supplementary file 1 [file Supplementary_resubmit.pdf]

# Supplementary material

# Why $Fe_3GaTe_2$ has higher Curie temperature than $Fe_3GeTe_2$?

Bomin Kim[1], Tumentsereg Ochirkhuyag[2], Dorj Odkhuu[2,*] and S. H. Rhim[1†]

[1]*Department of Physics, University of Ulsan, Ulsan 44610, Republic of Korea*

[2]*Department of Physics, Incheon National University, Incheon 22012, Republic of Korea*

**Contents**

I. Band analysis for $E_{\mathrm{MCA}}$: Te contribution 2

II. Mean-field model for three magnetic sublattices system 2

III. The hybridization mediated exchange 3

References 6

* odkhuu@inu.ac.kr

† sonny@ulsan.ac.kr

## I. Band analysis for $E_{\mathrm{MCA}}$: Te contribution

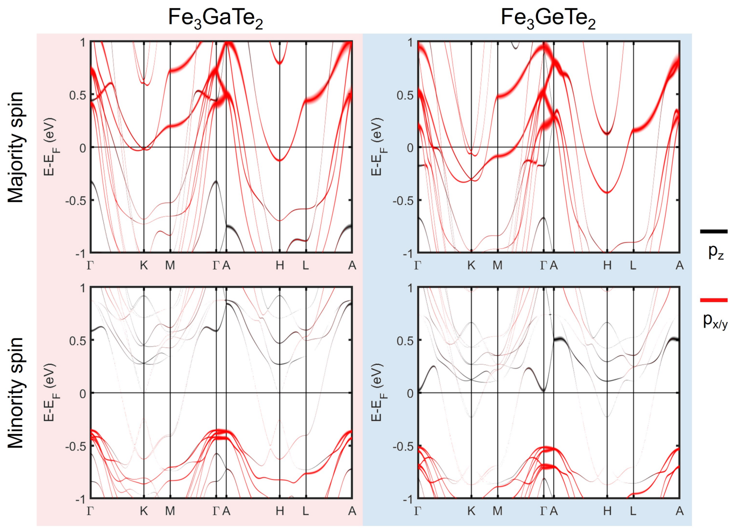


FIG. S1. Band structures of Te in $p$ orbital projection. $Fe_3GaTe_2$ and $Fe_3GeTe_2$ in red box and blue box, respectively. Upper (lower) panels for the majority (minority) spin channel. $p$ orbital decomposition into $p_z$ (black line) and $p_{x/y}$ (red line) according to the irreducible representation of hexagonal symmetry.

Te shows a larger $E_{\mathrm{MCA}}$ in $Fe_3GeTe_2$ compared to $Fe_3GaTe_2$. Fig. S1 shows band structures of Te, where $p$ orbitals are decomposed into the irreducible representations $p_z$ (black line), and $p_{x/y}$ (red line). In Fig. S1, red (blue) box denotes $Fe_3GaTe_2$ ($Fe_3GeTe_2$); upper (lower) panels are for the majority (minority) spin channel. In both structures, $E_{\mathrm{MCA}} > 0$ mainly comes from $\langle p_{x/y},\uparrow|L_z|p_{x/y},\uparrow\rangle$. In the majority spin channel of $Fe_3GaTe_2$, bands with relatively higher weights are in the unoccupied state, while bands with lower weights are in the occupied state. In $Fe_3GeTe_2$, bands with higher weights become occupied near $M\Gamma$. Therefore, although the same matrix $\langle p_{x/y},\uparrow|L_z|p_{x/y},\uparrow\rangle$ gives $E_{\mathrm{MCA}} > 0$ for both structures, $Fe_3GeTe_2$ has a larger value due to the higher orbital weight of the bands in the occupied state.

## II. Mean-field model for three magnetic sublattices system

In the mean-field approximation, the Curie temperature ($T_C$) for one magnetic sublattice system is expressed as

$$T_C \approx \frac{1}{k_B} z J_1, \tag{1}$$

where $k_B$ is the Boltzmann constant; $z$ is the number of first nearest neighbors; $J_1$ is the exchange coefficients of the nearest neighbor. For a Ising magnet with two magnetic sublattices $A$ and $B$, the interaction matrix of the Hamiltonian gives eigenvalue equation [1]

$$\begin{vmatrix} x-J_{AA} & -J_{AB} \\ -J_{AB} & x-J_{BB} \end{vmatrix} = 0, \tag{2}$$

where $x$ is $k_BT$; $J_{AA}$ and $J_{BB}$ are the intra-sublattice exchange constants for sublattice $A$ and $B$, respectively; $J_{AB}$ represents the inter-sublattice interaction. For simplicity, the number of all interactions is set to unity one ($z$=1) without loss of generality. By diagonalizing this 2×2 matrix, eigenvalues are obtained

$$T_C = \frac{1}{2k_B}(J_{AA}+J_{BB}) + \frac{1}{2k_B}\sqrt{(J_{AA}-J_{BB})^2+4J_{AB}^2}. \tag{3}$$

As shown clearly, not only one $J$, but also two additional $J$ terms must be considered to get $T_C$. For the system with three magnetic sublattices $A$, $B$, and $C$, the $3\times3$ interaction matrix is

$$\begin{vmatrix} x-J_{AA} & -J_{AB} & -J_{CA} \\ -J_{AB} & x-J_{BB} & -J_{BC} \\ -J_{CA} & -J_{BC} & x-J_{CC} \end{vmatrix} = 0, \tag{4}$$

where $x$ is $k_BT$; $J_{AA}$, $J_{BB}$, and $J_{CC}$ are the intra-sublattice exchange constants for sublattice $A$, $B$, and $C$, respectively; $J_{AB}$, $J_{BC}$, and $J_{CA}$ are the inter-sublattice interactions. The secular equation, Eq.4 becomes

$$\begin{aligned} x^3 - (J_{AA}+J_{BB}+J_{CC})x^2 - (J_{AB}^2+J_{BC}^2+J_{CA}^2-J_{AA}J_{BB}-J_{CC}J_{AA}-J_{BB}J_{CC})x \\ -J_{AA}J_{BB}J_{CC} - 2J_{AB}J_{BC}J_{CA} + J_{AA}J_{BC}^2 + J_{BB}J_{CA}^2 + J_{CC}J_{AB}^2 = 0. \end{aligned} \tag{5}$$

The cubic equation, Eq.5, requires six $J$ terms. In general, the cubic equation is solved using Cardano's formula, giving $T_C$ of $Fe_3GaTe_2$ and $Fe_3GeTe_2$. By this way, we obtain eigenvalues for $Fe_3GaTe_2$ 307.63, 307.63, and $1.31\times10^{-18}$; for $Fe_3GeTe_2$, 219.66, $3.82\times10^9$, and $3.82\times10^9$. These results, 307.63 K and 219.66 K, are close to the experimental results, 380 K and 230 K, for $Fe_3GaTe_2$ and $Fe_3GeTe_2$, respectively.

### III. The hybridization mediated exchange

The opposite signs of higher order $J$ in $Fe_3GaTe_2$ and $Fe_3GeTe_2$ are analyzed. More specifically we focus on the opposite signs of $J_3$ and $J_3'$ based on hybridization mediated exchange

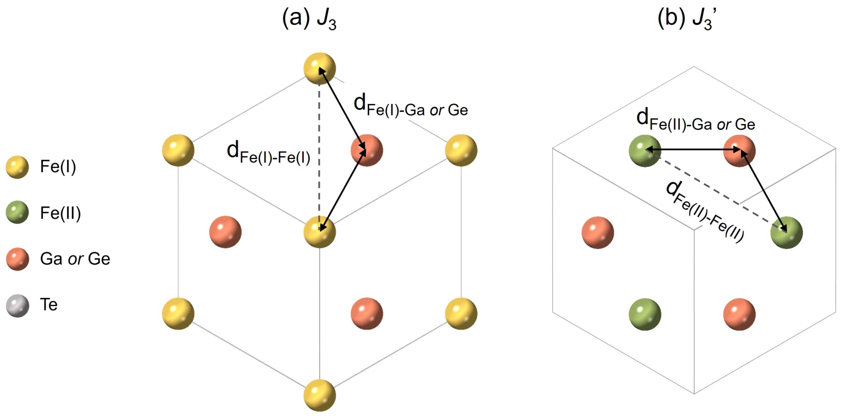


(c)

| | $J_3$ | | $J_3$' | |
|---|---|---|---|---|
| | $d_{\text{Fe(I)-Fe(I)}}$ | $d_{\text{Fe(I)-Ga } or \text{ Ge}}$ | $d_{\text{Fe(II)-Fe(II)}}$ | $d_{\text{Fe(II)-Ga } or \text{ Ge}}$ |
| $Fe_3GaTe_2$ | 4.03 Å | 2.62 Å | 4.03 Å | 2.33 Å |
| $Fe_3GeTe_2$ | 4.02 Å | 2.63 Å | 4.02 Å | 2.32 Å |

FIG. S2. The top view of the structures for (a) $J_3$ and (b) $J_3'$ shows only the atoms involved in each exchange interaction for better visibility. The distances between atoms are shown in (c), the Fe-Ga/Ge distances are shorter than the Fe-Fe distances.

model, similar to conventional super-exchange model. The hybridization of Fe-Ga/Ge is justified by partial density of states (PDOS) analysis. While the original super-exchange model assumes electronic hopping via ligand atoms, here the hybridization of Fe-Ga/Ge replaces simple-minded hopping with covalent feature of $Fe_3Ga/GeTe_2$.

For $J_3$ and $J_3'$, Fe atoms are far away, distance exceeding 4 $\AA$. Fig. S2 shows atoms relevant for $J_3$ and $J_3'$ for better visibility, where atom-atom distances are listed in Fig. S2 (c). Clearly, Fe-Ga/Ge distances are much shorter than Fe-Fe ones. Hence, the exchange interaction between Fe-Fe characterized as $J_3$ and $J_3'$ are of indirect exchange interaction mediated by Ga/Ge by Fe-Ga/Ge hybridization.

Fig. S3 shows schematics of the exchange interaction between Fe for (a) $Fe_3GaTe_2$ and (b) $Fe_3GeTe_2$. As we said, the Fe-Fe exchange interaction is mediated by hybridization with Ga or Ge due to atomic distances. Nominal valency of Fe is $d^6$, which is good approximation considering 6.3 electrons for Fe $d$ orbital from our calculations; nominal valency of Ga and Ge are $p^1$ and $p^2$, respectively. Due to hexagonal symmetry, $d$ orbitals are split into $m = 0, \pm1, \pm2$; $p$ orbital into $m = 0, \pm1$. For $Fe_3GaTe_2$ [Fig. S3 (a)], parallel spin configuration is possible by Fe-Ga hybridization. Hence, $J_3$ and $J_3'$ in $Fe_3GaTe_2$ prefer positive signs. On the other hand, for $Fe_3GeTe_2$

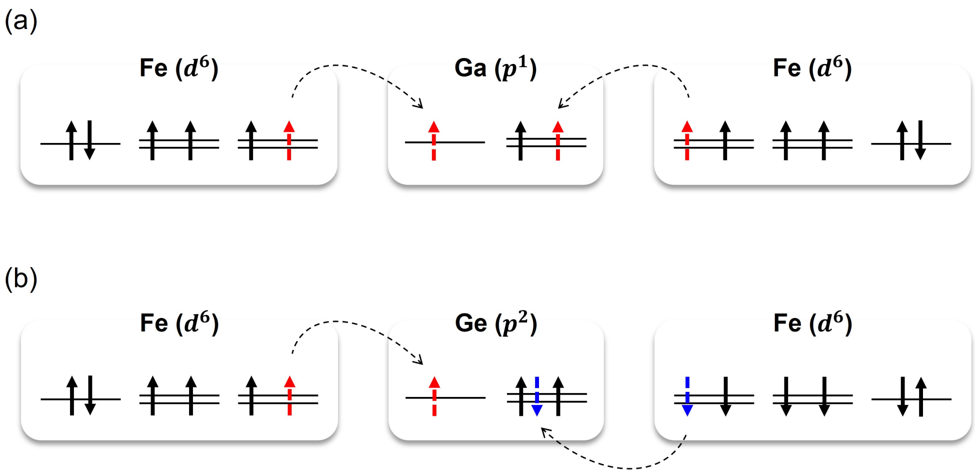


FIG. S3. Schematics of the exchange interactions between Fe in (a) $Fe_3GaTe_2$ and (b) $Fe_3GeTe_2$, mediated by Ga or Ge. Since Ga has $p^1$, Fe can share parallel spin in $Fe_3GaTe_2$, but as Ge has $p^2$, Fe shares antiparallel spin instead in $Fe_3GeTe_2$.

[Fig. S3 (b)], as $p^2$ states, split by crystal field, has no room, parallel spin configuration is not allowed owing to Pauli exclusion principle. Hence, antiparallel spin configurations are possible, hence $J_3$ and $J_3'$ in $Fe_3GeTe_2$ prefer negative signs.

To confirm our argument, PDOS analysis is performed for orbital resolved $J_3$. Figs. S4 (a)-(d) present PDOS, where left and right panels for $Fe_3GaTe_2$ and $Fe_3GeTe_2$, respectively; while upper and lower panels show Fe(I) and Ga/Ge, respectively. $d$ and $p$ orbitals are denoted by solid and dashed lines, respectively; important peaks are labeled by $A_1$, $A_2$, $B_1$, $B_2$, and their variants. In the majority spin state, $A_1$ and $A_1'$ of Fe(I) $d_{xz/yz}$ and Ga $p_z$ in $Fe_3GaTe_2$ are hybridized and partially occupied. Similarly, in $Fe_3GeTe_2$, $A_2$ and $A_2'$ of Fe(I) $d_{xz/yz}$ and Ge $p_z$ are also hybridized and partially occupied. In the minority spin state, $B_1$ and $B_1'$ of Fe(I) $d_{x^2-y^2/xy}$ and Ga $p_z$ in $Fe_3GaTe_2$ are hybridized and unoccupied. On the other hand, in $Fe_3GeTe_2$, $B_2$ and $B_2'$ of Fe(I) $d_{x^2-y^2/xy}$ and Ge $p_z$ are hybridized and partially occupied. These differences of the occupation in the minority spin state of Fe(I) between two structures are consistent with the analysis of magneto-crystalline anisotropy presented in the main manuscript.

Fig. S4 (e) and (f) show the orbital resolved $J_3$ in $Fe_3GaTe_2$ and $Fe_3GeTe_2$, respectively. $Fe_3GaTe_2$ exhibits a large $J > 0$ from $d_{xz/yz} - d_{xz/yz}$ interactions, while $Fe_3GeTe_2$ shows a large $J < 0$ from $d_{x^2-y^2/xy} - d_{x^2-y^2/xy}$ interactions. Due to different occupation as well as hybridization with Ga/Ge, as described above, $J_3$ in $Fe_3GaTe_2$ and $Fe_3GeTe_2$ exhibit different signs and orbital

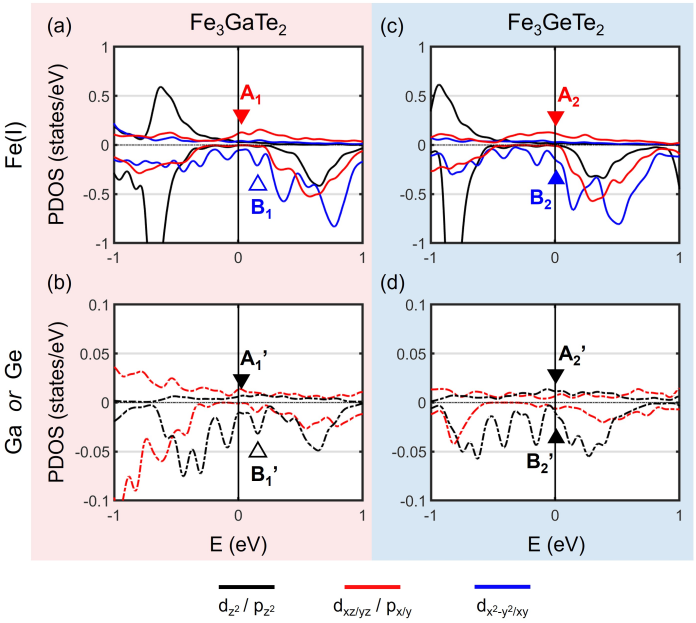


(e) $J_3$ in $Fe_3GaTe_2$

| [meV] | $d_{z^2}$ | $d_{xz/yz}$ | $d_{x^2-y^2/xy}$ |
|---|---|---|---|
| $d_{z^2}$ | −0.05 | −0.64 | 0.16 |
| $d_{xz/yz}$ | −0.64 | 6.08 | −0.52 |
| $d_{x^2-y^2/xy}$ | 0.16 | −0.52 | −0.56 |

(f) $J_3$ in $Fe_3GeTe_2$

| [meV] | $d_{z^2}$ | $d_{xz/yz}$ | $d_{x^2-y^2/xy}$ |
|---|---|---|---|
| $d_{z^2}$ | −0.09 | −0.60 | 0.01 |
| $d_{xz/yz}$ | −0.60 | 0.62 | −0.10 |
| $d_{x^2-y^2/xy}$ | 0.01 | −0.10 | −2.41 |

FIG. S4. Partial density of states of (a) Fe(I) and (b) Ga in $Fe_3GaTe_2$, (c) Fe(I) and (d) Ge in $Fe_3GeTe_2$. Orbital resolved $J_3$ in (e) $Fe_3GaTe_2$ and (f) $Fe_3GeTe_2$. $Fe_3GaTe_2$ exhibits a large positive $J$ value from $d_{xz/yz}$-$d_{xz/yz}$ interactions, while $Fe_3GeTe_2$ shows a large negative $J$ value from $d_{x^2-y^2/xy}$-$d_{x^2-y^2/xy}$ interactions.

contributions.

---

[1] R. Skomski, *Simple models of magnetism* (Oxford University Press, 2008).
